# Supplementary material for: FileInsurer: A Scalable and Reliable Protocol for Decentralized File Storage in Blockchain
Source: arXiv:2207.11657 source file (2022-07-24)
Supplement: Supplementary file 1 [file experiment_appendix.tex]

\section{experiment}
\label{experiment}
\hy{different size of sectors}
Recall that $N_{cp}=kN_v$ is the number of file backups and each file $f$ needs to store $f.cp$ backups on the network. \Cref{table:experiment} shows the result of the capacity usage of the most loaded sector in the experiment. We run the experiment under two different settings. In the first setting, we reallocate all file backups in one go for $100$ times. In the second setting, we allocate each file backup and then randomly refresh the location of a file backup $100N_{cp}$ times. In the experiment, we record the maximum value of capacity usage at any time. The results are shown in \cref{table:experiment}. That the maximum capacity usage is less than $1$ means that no file backups are allocated to sectors with insufficient capacity.
We can find that under the distributions we test in the experiments, the probability of that file backups are allocated to sectors with insufficient capacity is sufficiently small.
\begin{table}[]
    \caption{\textbf{Experiment result:} maximum capacity usage of sectors}
    \centering{\small
    \begin{tabular}{c c|c c c c c}
        \hline\hline
        \multicolumn{7}{c}{reallocate all file backups $100$ times} \
        \cr \cline{1-7}
        \multicolumn{2}{c}{parameter} & \multicolumn{5}{c}{maximum capacity usage} \
        \cr \cline{1-2} \cline{3-7}
        $N_{cp}$ & $N_s$ & $[1]$ & $[2]$ & $[3]$ & $[4]$ & $[5]$\\
        \hline
$10^5$ & 5 & 0.511 & 0.508 & 0.514 & 0.511 & 0.509\\\hline
$10^5$ & 10 & 0.519 & 0.518 & 0.521 & 0.518 & 0.515\\\hline
$10^5$ & 20 & 0.525 & 0.524 & 0.536 & 0.530 & 0.529\\\hline
$10^5$ & 50 & 0.565 & 0.539 & 0.558 & 0.549 & 0.548\\\hline
$10^5$ & 100 & 0.571 & 0.566 & 0.584 & 0.572 & 0.569\\\hline
$10^6$ & 50 & 0.515 & 0.513 & 0.517 & 0.515 & 0.513\\\hline
$10^6$ & 100 & 0.522 & 0.523 & 0.530 & 0.530 & 0.521\\\hline
$10^6$ & 200 & 0.538 & 0.530 & 0.542 & 0.534 & 0.533\\\hline
$10^6$ & 500 & 0.558 & 0.548 & 0.569 & 0.570 & 0.557\\\hline
$10^6$ & 1000 & 0.591 & 0.571 & 0.598 & 0.594 & 0.576\\\hline
$10^7$ & 500 & 0.516 & 0.515 & 0.522 & 0.521 & 0.518\\\hline
$10^7$ & 1000 & 0.524 & 0.521 & 0.531 & 0.528 & 0.524\\\hline
$10^7$ & 2000 & 0.540 & 0.534 & 0.544 & 0.545 & 0.534\\\hline
$10^7$ & 5000 & 0.562 & 0.554 & 0.581 & 0.573 & 0.560\\\hline
$10^7$ & 10000 & 0.589 & 0.576 & 0.609 & 0.606 & 0.585\\\hline
$10^8$ & 5000 & 0.520 & 0.518 & 0.522 & 0.520 & 0.517\\\hline
$10^8$ & 10000 & 0.526 & 0.525 & 0.537 & 0.529 & 0.524\\\hline
$10^8$ & 20000 & 0.541 & 0.534 & 0.550 & 0.547 & 0.538\\\hline
$10^8$ & 50000 & 0.562 & 0.555 & 0.580 & 0.571 & 0.559\\\hline
$10^8$ & $10^5$ & 0.591 & 0.582 & 0.614 & 0.599 & 0.586\\\hline
        \hline
    \end{tabular}
    \begin{tabular}{c c|c c c c c}
        \hline\hline
        \multicolumn{7}{c}{refresh the location of a file backup $100N_{cp}$ times} \
        \cr \cline{1-7}
        \multicolumn{2}{c}{parameter} & \multicolumn{5}{c}{maximum capacity usage} \
        \cr \cline{1-2} \cline{3-7}
        $N_{cp}$ & $N_s$ & $[1]$ & $[2]$ & $[3]$ & $[4]$ & $[5]$\\
        \hline
$10^5$ & 5 & 0.517 & 0.511 & 0.519 & 0.515 & 0.514\\\hline
$10^5$ & 10 & 0.524 & 0.523 & 0.529 & 0.522 & 0.519\\\hline
$10^5$ & 20 & 0.532 & 0.529 & 0.538 & 0.535 & 0.531\\\hline
$10^5$ & 50 & 0.550 & 0.551 & 0.566 & 0.554 & 0.557\\\hline
$10^5$ & 100 & 0.588 & 0.571 & 0.599 & 0.595 & 0.581\\\hline
$10^6$ & 50 & 0.518 & 0.516 & 0.521 & 0.519 & 0.517\\\hline
$10^6$ & 100 & 0.525 & 0.522 & 0.532 & 0.529 & 0.526\\\hline
$10^6$ & 200 & 0.536 & 0.535 & 0.546 & 0.542 & 0.541\\\hline
$10^6$ & 500 & 0.565 & 0.563 & 0.582 & 0.575 & 0.562\\\hline
$10^6$ & 1000 & 0.592 & 0.581 & 0.610 & 0.605 & 0.589\\\hline
$10^7$ & 500 & 0.520 & 0.518 & 0.525 & 0.523 & 0.522\\\hline
$10^7$ & 1000 & 0.533 & 0.527 & 0.534 & 0.533 & 0.531\\\hline
$10^7$ & 2000 & 0.542 & 0.535 & 0.553 & 0.549 & 0.540\\\hline
$10^7$ & 5000 & 0.565 & 0.562 & 0.586 & 0.582 & 0.569\\\hline
$10^7$ & 10000 & 0.610 & 0.591 & 0.626 & 0.613 & 0.599\\\hline
$10^8$ & 5000 & 0.529 & 0.527 & 0.539 & 0.532 & 0.529\\\hline
$10^8$ & 10000 & 0.542 & 0.536 & 0.543 & 0.546 & 0.537\\\hline
$10^8$ & 20000 & 0.551 & 0.547 & 0.560 & 0.558 & 0.548\\\hline
$10^8$ & 50000 & 0.575 & 0.569 & 0.599 & 0.584 & 0.577\\\hline
$10^8$ & $10^5$ & 0.611 & 0.604 & 0.639 & 0.628 & 0.611\\\hline
        \hline
    \end{tabular}}
    \begin{tablenotes}
      \footnotesize
      \item $[1]$: Uniform distribution in interval $[0,1]$
      \item $[2]$: Uniform distribution in interval $[1,2]$
      \item $[3]$: Exponential distribution
      \item $[4]$: Normal distribution with $\mu = \sigma^2$
      \item $[5]$: Normal distribution with $\mu = 2\sigma^2$
    \end{tablenotes}
    \label{table:experiment}
\end{table}
